# Supplementary material for: Disruptive Autoencoders: Leveraging Low-level features for 3D Medical Image Pre-training
Source: arXiv:2307.16896 source file (2023-07-31)

Current Work

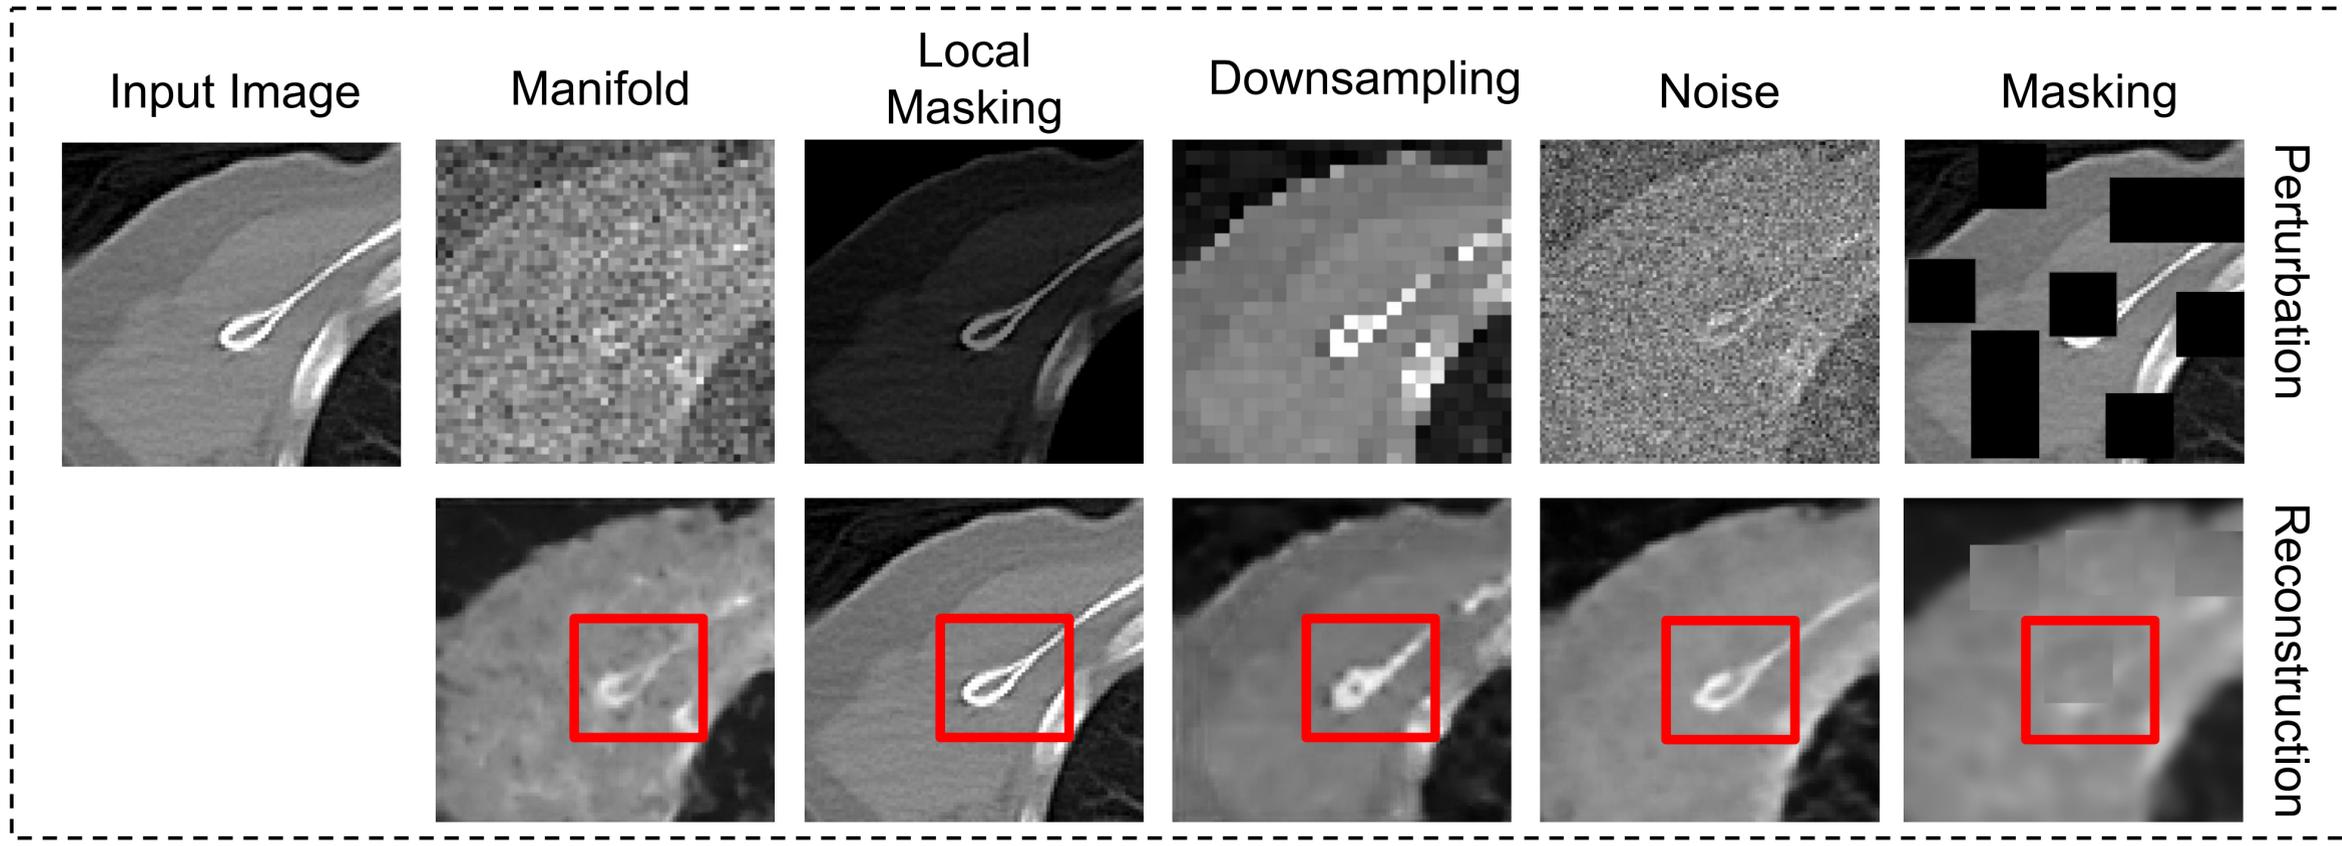

Reconstruction Masking Input Image

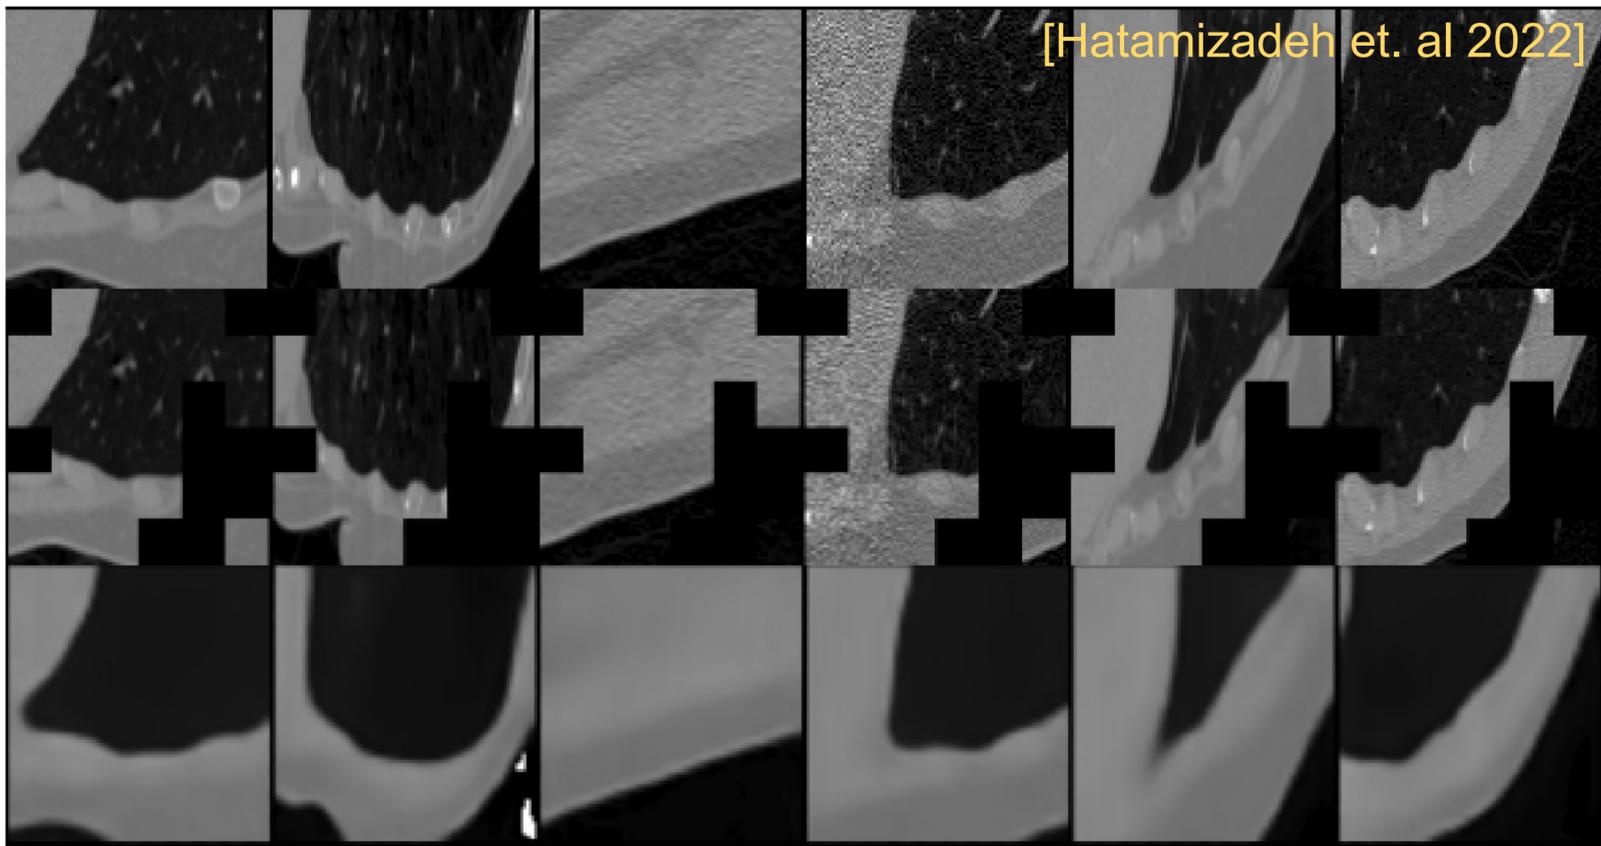

Reconstruction Masking Input Image

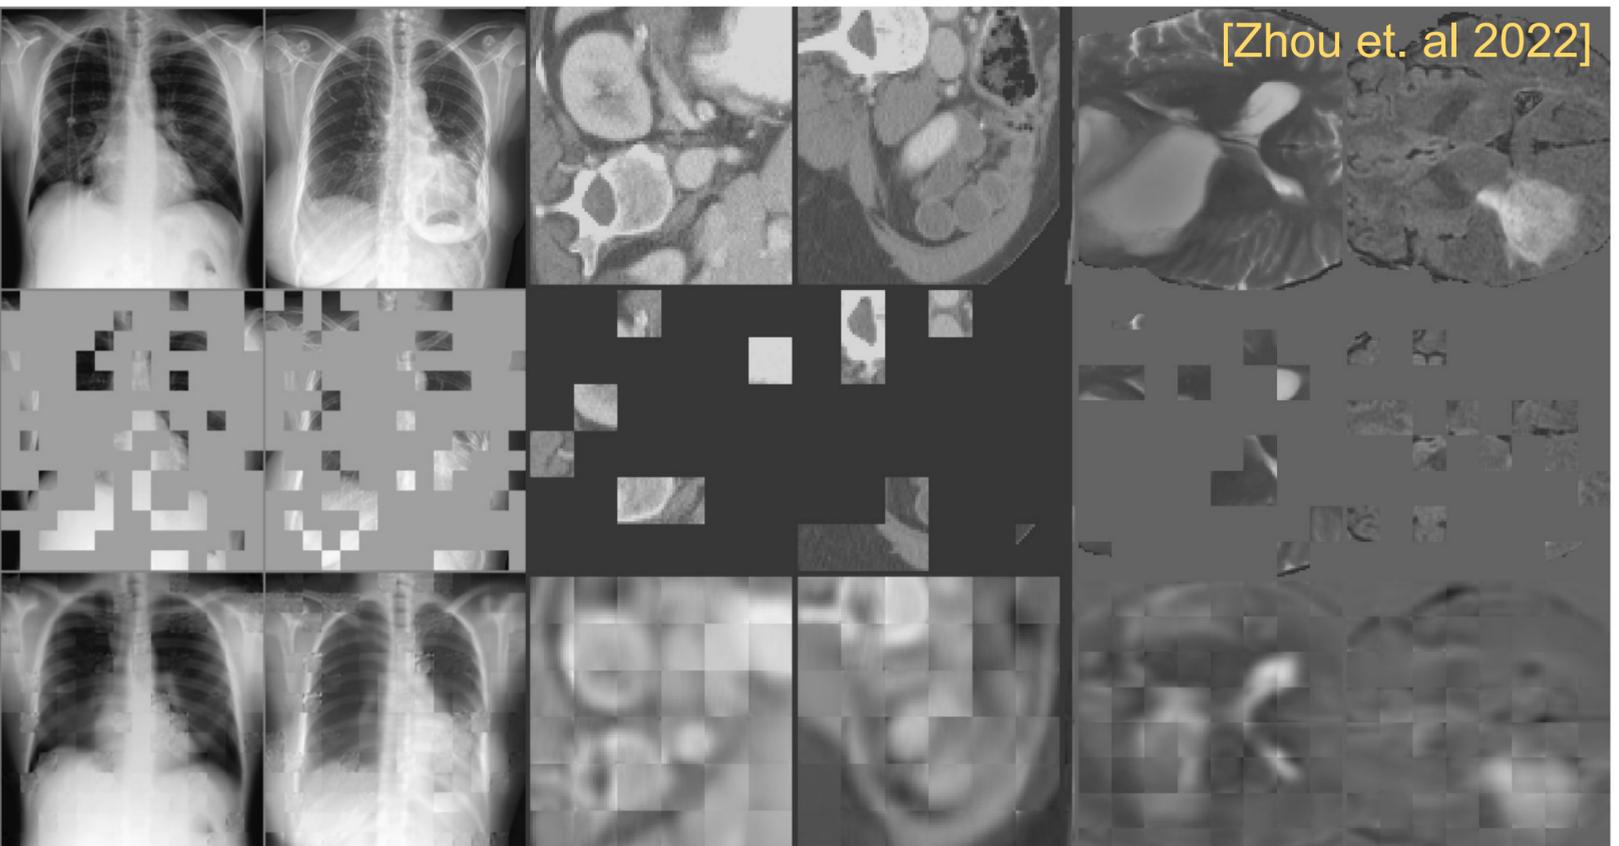

Current Work

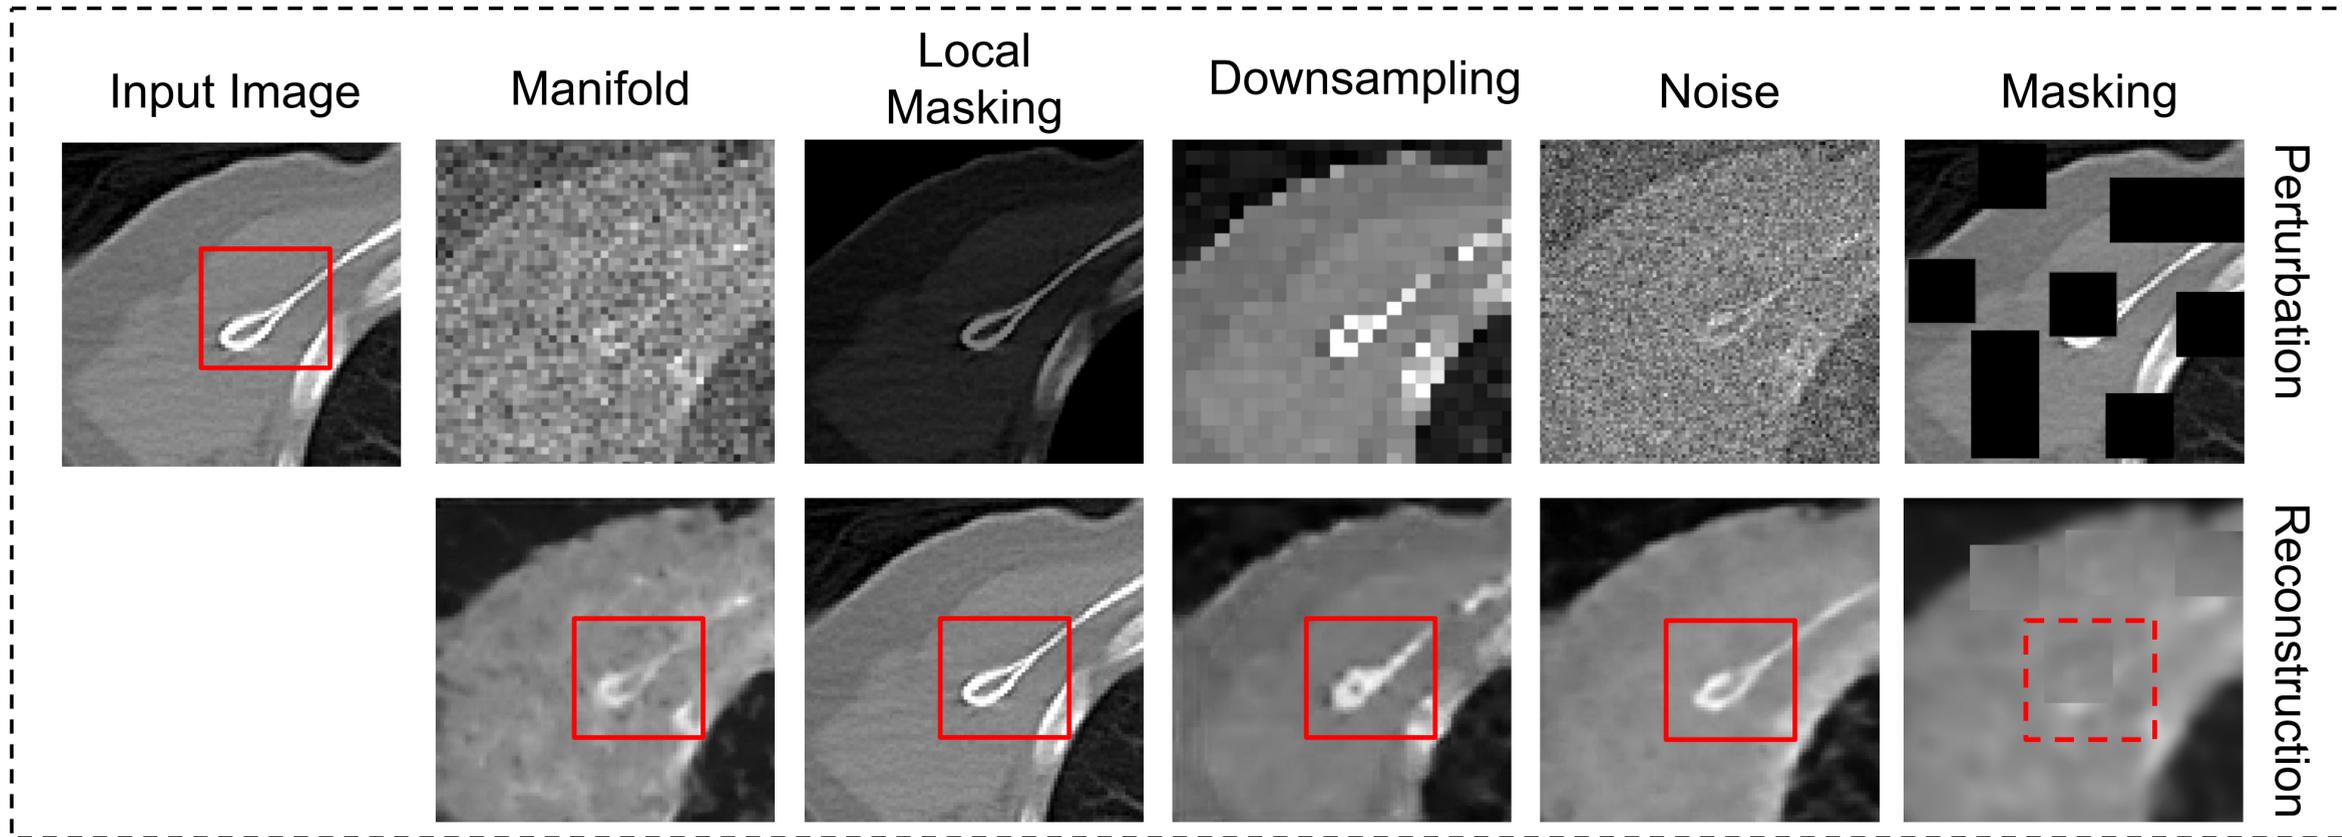

Reconstruction    Masking    Input Image

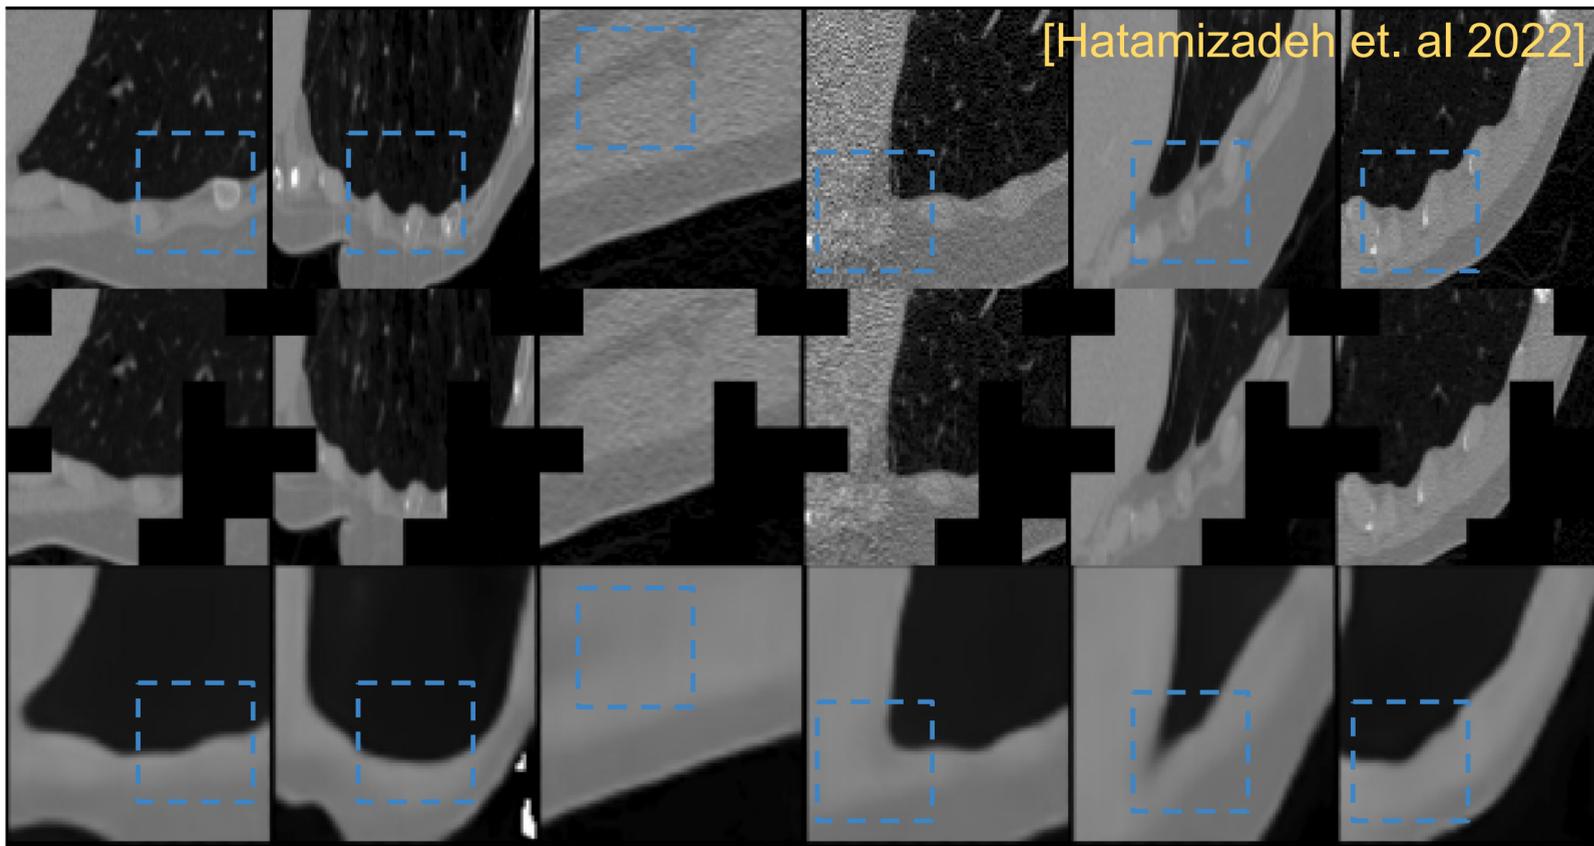

Reconstruction    Masking    Input Image

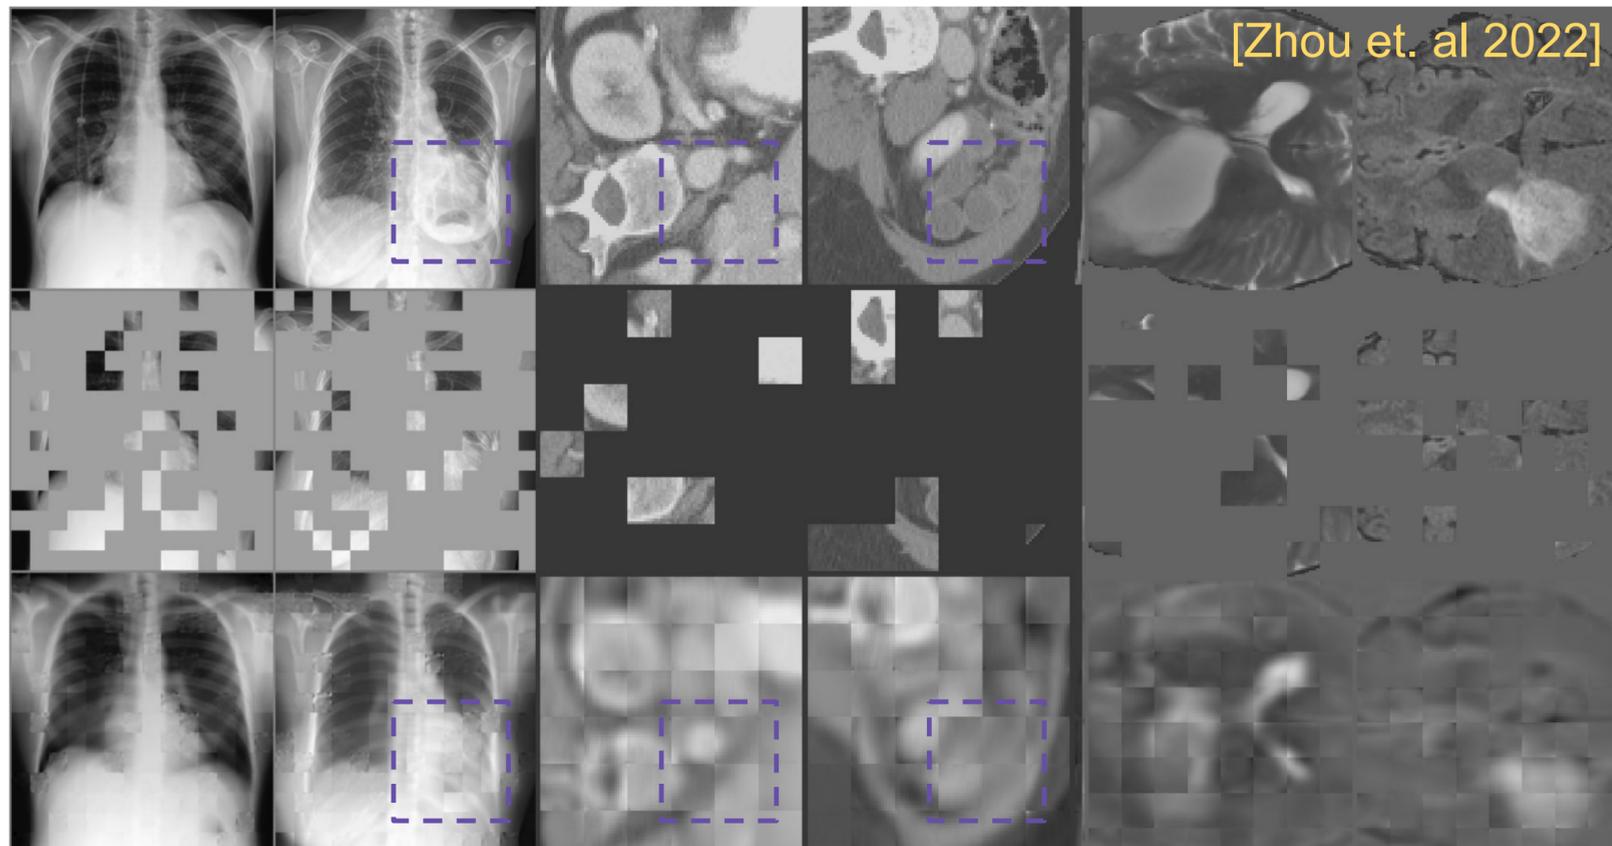

Supplement: Supplementary file 1 [file Supple_Recon_Prior_Work_Comparison_Fig.pdf]
